# Supplementary material for: Instructify: Demystifying Metadata to Visual Instruction Tuning Data Conversion
Source: arXiv:2505.18115 source file (2025-05-23)
Supplement: Supplementary file 1 [file supp_prompt_shikra.tex]

\begin{figure*}[ht]
% \vspace{-0.3cm}
\centering
\includegraphics[width=0.95\linewidth]{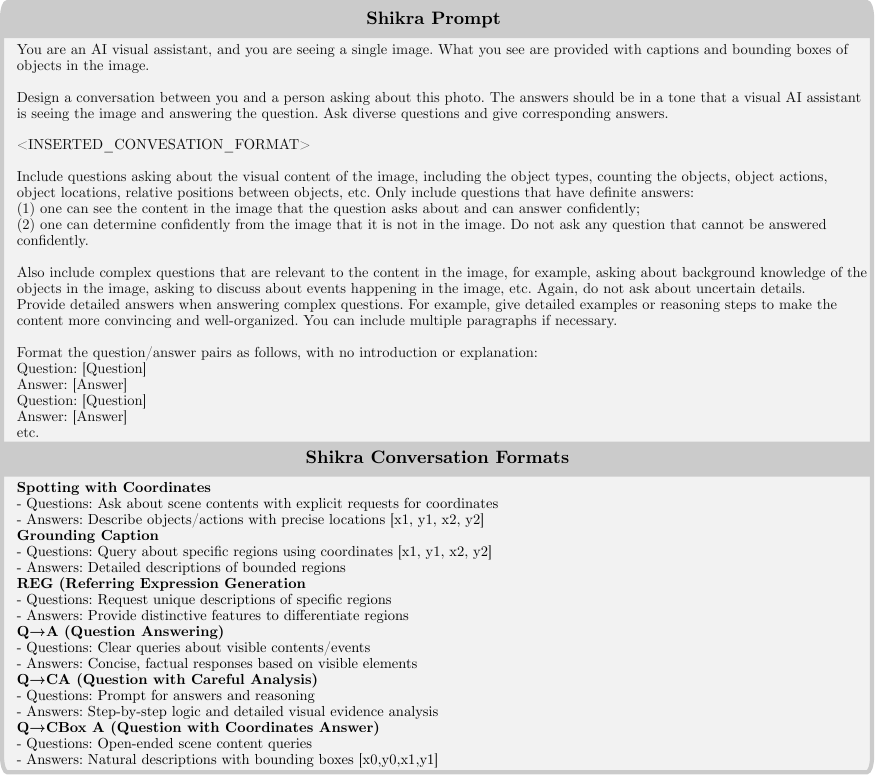}
\caption{
\label{fig:prompt_shikra}
\textbf{Shikra prompt.}
}
\end{figure*}
